# Supplementary material for: Finite- and Large- Sample Inference for Model and Coefficients in High-dimensional Linear Regression with Repro Samples
Source: arXiv:2209.09299 source file (2025-11-27)
Supplement: Supplementary file 1 [file Appendix_additional_simulation.tex]

{
%\color{red} add to paper}
% In this section, we present simulation results for two additional challenging settings (M4) and (M5), besides (M1)-(M3) presented in Section~\ref{sec:simulation}.
\begin{itemize}
    \item[(M4)] 
     (Perfect colinearity, restricted eigenvalue conditions not satisfied )
	 {Let $\bbeta_0^{full}=(3, 2, 1.5, 0, \dots, 0)$.}  For $j_1,j_2\in[p]$, the correlation between $x_{j_1}$ and $x_{j_2}$ is set to $0.5^{|j_1 - j_2 |}$. To create perfect colinearity, make $2x_10 + 3x_{11} + x_{10} = 3x_{1} + 2x_{2} + 1.5x_{3},$ such that the restricted eigenvalue conditions do not hold, and $C_{\min} = 0.$ 
 We set $n = 50,p = 1000$ and $\sigma = 1$.

\item[(M5)] (From \cite{li_model_2019}, low dimensional setting, but with many signals) Let $\bbeta_0^{full}=(\underbrace{1, \dots, 1}_{12}, 0, \dots, 0).$ For $j_1,j_2\in[p]$, the correlation between $x_{j_1}$
and $x_{j_2}$ is set to $0.5^{|j_1 - j_2 |}$. We let %$n = 300,$ 
$n = 150$, 
$p = 200$ and $\sigma = 1$.
\end{itemize}

\begin{table}[ht]
\caption{Repro Confidence Sets for True Model $\tau_0$}
\label{tab:mod_confidence_sets_appendix}
\scriptsize
\begin{tabular}{ll|ll}
\hline
 & {Method} & Cardinality of $\Gamma^{\tau}_{0.95}$& Coverage of $\Gamma^{\tau}_{0.95}$ \\
 \hline
\multirow{4}{*}{\shortstack{Model M4: $n=50, p=1000$\\ Perfect Colinearity  %\\  %$d=1,000$
}} & Repro samples &  2.640 (0.164)  & 0.985 (0.009) \\
                  & Bootstrap AIC  & 57.875 (6.820)  & 0.000 (0.000)  \\
                  & Bootstrap BIC & 41.410 (5.191)  & 0.000 (0.000)   \\
                  & Bootstrap CV &74.065 (7.925)  & 0.000 (0.000)   \\
                  \hline
\multirow{4}{*}{\shortstack{Model M5: $n=300, p=200$\\ From \cite{li_model_2019}, 12 signals %\\  % $d=10,000$
}} & Repro samples &1.010 (0.007)     & 1.000 (0.000)  \\
                  & Bootstrap AIC  & 601.645 (12.612) & 1.000 (0.000)  \\
                  & Bootstrap BIC &   246.995 ( 4.404)  & 1.000 (0.000)  \\
                  & Bootstrap CV &  567.150 (12.446)  & 1.000 (0.000)   \\
                  \hline
\end{tabular}
\end{table}

\begin{table}[ht]
\caption{Repro Confidence Sets for (Scalar) Regression Parameter $\beta_{0,i}$ with Comparison to Debiased LASSO}
\label{tab:confidence_interval_appendix}
\scriptsize
\begin{tabular}{lr|cc|cc|cc}
\hline
 & & \multicolumn{2}{c|}{Repro Samples}    & \multicolumn{2}{c|}{Debiased LASSO (JM) } & \multicolumn{2}{c}{Debiased LASSO (ZZ)}    \\ 
Model &  $\beta_{0,i}$ & Coverage & Width& Coverage & Width &  Coverage & Width   \\ \hline
\multirow{3}{*}{M4} & All $\beta_{0,i} $ & 1.000(0.000)  & 0.003(0.000)    & 0.984(0.000)  & 0.244(0.000) & NA  & NA \\
 & $\beta_{0,i} \neq 0$    & 0.953(0.009)     & 0.755(0.006)    & 0.337(0.019)     & 0.246(0.005) &   NA  &  NA  \\
 & $\beta_{0,i} = 0$      & 1.000(0.000)   & 0.001(0.000)    & 0.986(0.000)   & 0.244(0.000)  &  NA &  NA    \\
\hline
\multirow{3}{*}{M5}  & All $\beta_{0,i} $ &  0.998(0.000)  & 0.018(0.000) &0.971(0.001)  & 0.320(0.000) & 0.964(0.001)  & 0.339(0.000)  \\
 & $\beta_{0,i} \neq 0$    & 0.960(0.004)     & 0.296(0.000)  &0.950(0.004)     & 0.319(0.001) &0.959(0.004)     & 0.338(0.000)   \\
 & $\beta_{0,i} = 0$       & 1.000(0.000)   & 0.000(0.000)   & 0.984(0.001)   & 0.498(0.000)  & 0.965(0.001)   & 0.339(0.000) \\
\hline
\end{tabular}
\end{table}

We summarized the results for 95\% model confidence sets in Table~\ref{tab:mod_confidence_sets_appendix}. In the challenging scenario of (M4), where no typical conditions in the existing literature are met, the bootstrap confidence set fail to cover the true model at all, a more severe issue than in (M1)-(M3). In these earlier simulation settings, despite their size, the bootstrap sets at least manage to cover $\tau_0$.  In contrast, the repro sample confidence sets maintained their excellent performance, covering the true model 98.5\% of the time with an average size of only 2.6 models. For (M5), a low dimensional setting where $p<n,$  the repro samples confidence set covers the $\tau_0$ with just a single model most of the times.  This performance is notably more efficient than the confidence intervals described in \cite{li_model_2019}, which require a confidence bound width encompassing at least 20\% of $p=300,$ or 50 variables to achieve the desired coverage rate.  The reliance of their confidence bounds approach on bootstrap techniques, which generate a large number of models as indicated in Table~\ref{tab:mod_confidence_sets_appendix}, contributes partly to their excessively broad confidence bounds.

In Table~\ref{tab:confidence_interval_appendix}, we compare the confidence intervals of a single regression coefficients between the repro samples method and the debiased lasso approach. First of all, for (M4), the debiased lasso approach (ZZ) by \cite{zhang_confidence_2014} does not provide results for most of the simulated data set due to the perfect colinearity between the covariates.  Compared to the debiased lasso approach (JM) in \cite{javanmard_confidence_2014}, the repro samples approach successfully achieves the desired coverage rates for both the zero coefficients and all the signals, while the debiased lasso fail to cover the signals with a coverage rate only 0.337.  For the low dimensional setting (M5), all methods manage to cover the true value of the regression coefficients with the desired coverage rate as expected.  In both (M4) and (M5), the repro samples confidence intervals are significantly narrower, except for the signals of (M4), for which the debiased approach severely undercover with a coverage rate of 0.337.
